# Supplementary material for: CUR Matrix Approximation through Convex Optimization for Feature Selection
Source: arXiv:2505.16032 ancillary file (2025-05-21)
Supplement: Supplementary file 1 [file CUR_Supplementary_Material.pdf]

# Supplementary Material

## 1 SF CUR and LS-D CUR Probe Selection

| # of Probes | # Distinct |
|-------------|------------|
| 5           | 0          |
| 10          | 0          |
| 15          | 0          |
| 20          | 1          |
| 25          | 1          |
| 30          | 2          |
| 35          | 2          |
| 40          | 2          |
| 45          | 1          |
| 50          | 2          |
| 55          | 3          |
| 60          | 4          |
| 65          | 3          |
| 70          | 4          |
| 75          | 3          |
| 80          | 3          |
| 85          | 4          |
| 90          | 5          |
| 95          | 7          |
| 100         | 7          |

Table S1: Number of distinct probes selected between SF CUR and LS-D CUR on gene expression data.

## 2 Discriminant Proteins Using CUR and BIC

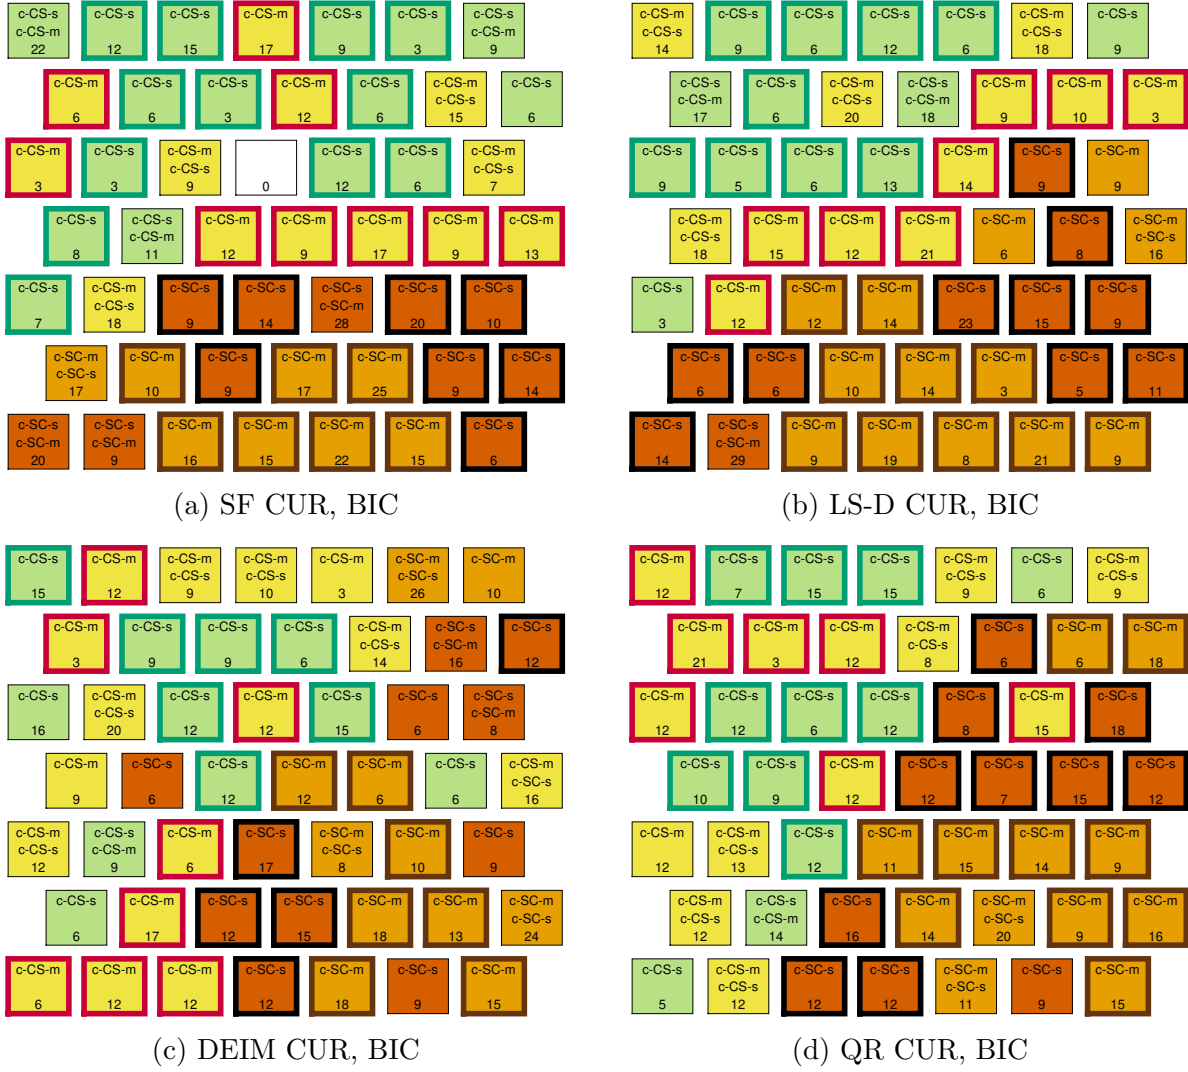

Figure S1: Experiment 1 discriminant protein SOMs for CUR algorithms using the BIC model selection criteria.

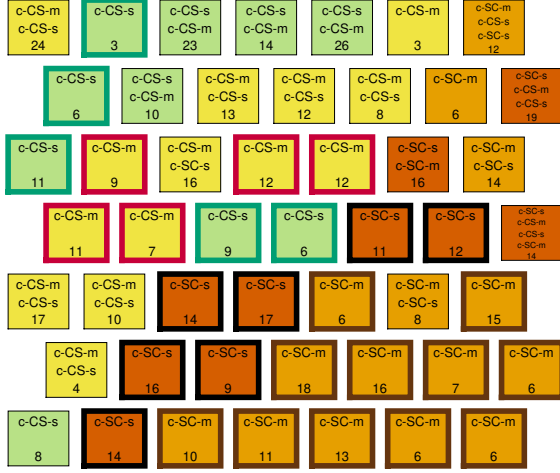

(a) SF CUR, BIC

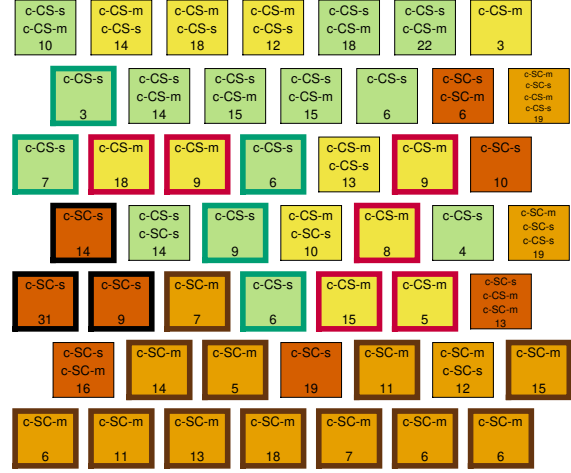

(b) LS-D CUR, BIC

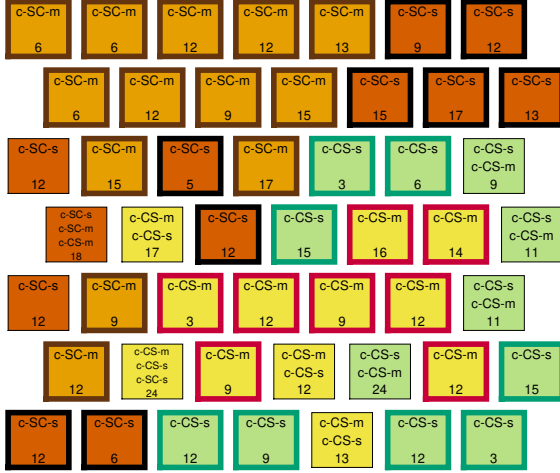

(c) DEIM CUR, BIC

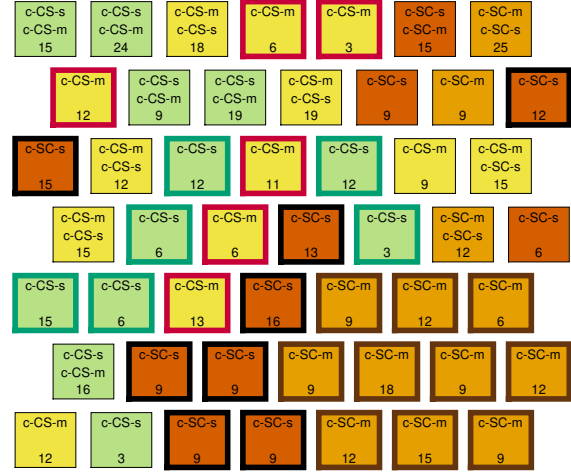

(d) QR CUR, BIC

Figure S2: Experiment 2 discriminant protein SOMs for CUR algorithms using the BIC model selection criteria.
